# Supplementary material for: Deep learning enabled strategies for modelling of complex aperiodic plasmonic metasurfaces of arbitrary size
Source: arXiv:2110.02109 ancillary file (2021-12-08)
Supplement: Supplementary file 1 [file 2021_majorel_supinfo.pdf]

# Supporting information: Deep learning enabled strategies for modelling of complex aperiodic plasmonic metasurfaces of arbitrary size

Clément Majorel,[1] Christian Girard,[1] Arnaud Arbouet,[1] Otto L. Muskens,[2] and Peter R. Wiecha[3,*]

[1]*CEMES-CNRS, Université de Toulouse, CNRS, UPS, Toulouse, France*
[2]*Physics and Astronomy, Faculty of Engineering and Physical Sciences, University of Southampton, Southampton, UK*
[3]*LAAS, Université de Toulouse, CNRS, Toulouse, France*

## A. Artificial Neural Network Details

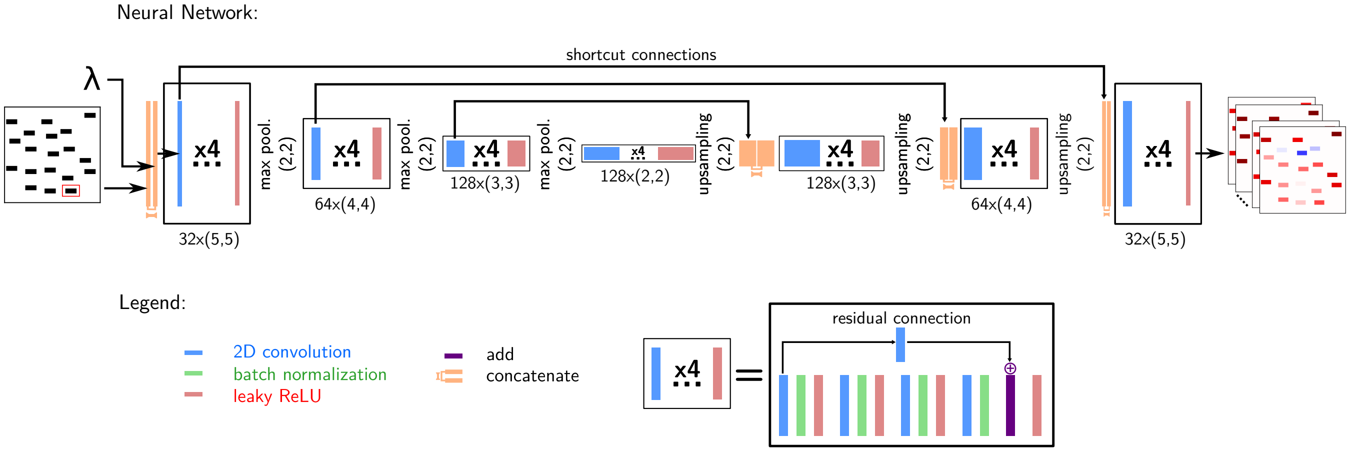


Figure S1. Detailed scheme of the network layout.

Each residual block of the network implements a series of 4 convolutional layers with a residual skip connection through an additional convolutional layer. Every convolution is followed by batch normalization[S1] and leaky ReLU activation[S2]. The center layer of the ANN is surrounded by 3 downsampling and 3 upsampling blocks, which decrease, respectively increase the image dimension each by a factor of 2. Downsampling is done by max pooling, upsampling by repetition. The first block consists of layer with 32 kernels, this number doubles after each pooling and reduces accordingly by halves in the up-sampling branch of the network. A sketch of the network layout with number and size of convolutional kernels is given in figure S1.

We train the ANN using the ADAM solver[S3] with a starting learning rate of 0.0001 and a batchsize of 16. We employ a training protocol with consecutively increasing batchsize, equivalent to a progressive reduction of the learning rate.[S4] We train the network for 200 epochs, which takes around 20 hours on our GPU. The training converges after around 100 epochs with no trace of overfitting (see also figure S4). Once training is finished, a prediction takes in the order of 2 ms on the same GPU, whereas the simulation takes in the order of 5 to 60 seconds, depending on the density of gold nanorods.

## B. Training data generation procedure

The process of training data generation is depicted in figure S2(a-b). We start the generation of a random structure with a regular array of positions with a randomly chosen particle density of between 10 and 60 rods per square micron. We then move each rod by a random vector within the structure plane. The largest possible shift is thereby limited to half the distance to the next gold-rod in the array (see figure S2a). In order to include also examples of partially covered areas, we truncate in 20% of the samples a part of the geometry at a randomly chosen $X$ or $Y$ position. This

* e-mail : pwiecha@laas.fr

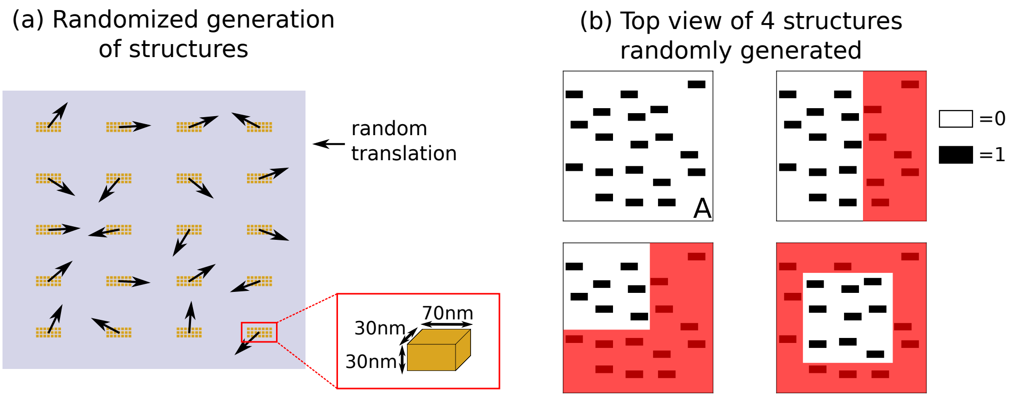


Figure S2. Procedure of data generation. (a) position randomization based on a regular grid. (b) in 80% of the cases, the full structure is kept (A). In 20% a random truncation is performed, removing structures at one or multiple sides of the area.

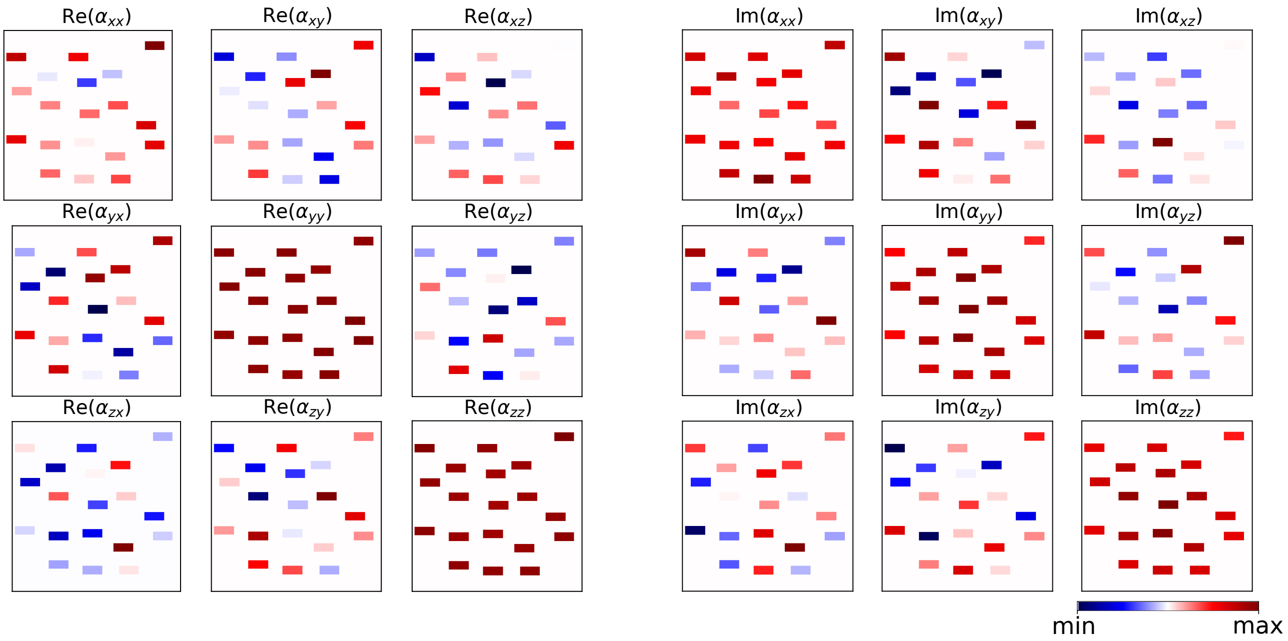


Figure S3. Full dressed polarizability tensor maps, as predicted by the neural network, here for the structure (A) shown in figure S2b. Left: real parts of the tensor components, right: according imaginary parts.

is done randomly for between one and all four sides of the area, as indicated by red shaded regions in figure S2b. This latter truncation procedure is in particular important so the network learns to correctly predict gold rods at border positions in the raster-scanning method. While we include only random structures based on the disordered grid-layout (with optional truncation), we found in systematic tests that the network manages well to generalize to ordered geometries such as the spiral or the perfect grid, shown the main text.

Before passing the data to the training, we normalize the polarizabilities to the maximum tensor norm in the data set, since the network cannot cope with the large values of the polarizabilities in units of nm$^3$.[S5] We note that in contrast to routine scaling procedures, we do not center the data around the mean value, because here the background of the predicted maps has a physical meaning – it corresponds to zero polarizability. Centering the data with respect to their average effectively requires the network to learn the mean value of the dataset for the background, which, first, is not a useful information, and second, we found that it reduces prediction fidelity.

To illustrate the amount of information which the neural network predicts, we shown in figure S3 the 18 output channels of the model, corresponding to 2D maps of the real and imaginary parts of the complex dressed polarizability tensor elements. Shown is the polarizability distribution for the structure “A” in figure S2b.

### C. Network details and training convergence

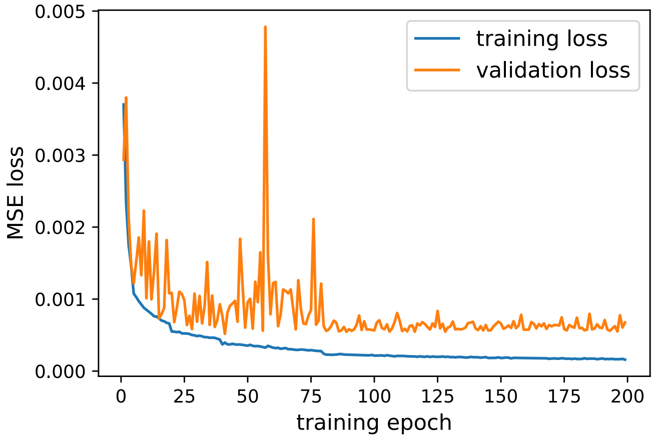


Figure S4. Training convergence. The validation loss (orange line) is noisy because validation is done on a small set of only 1000 samples (65000 samples for training). No trace of overfitting is observed.

We train the network for 200 epochs, but convergence is obtained already after around 100 epochs. No overfitting is observed, as can be seen in the training convergence plot, shown in figure S4.

### D. Error maps for prediction examples

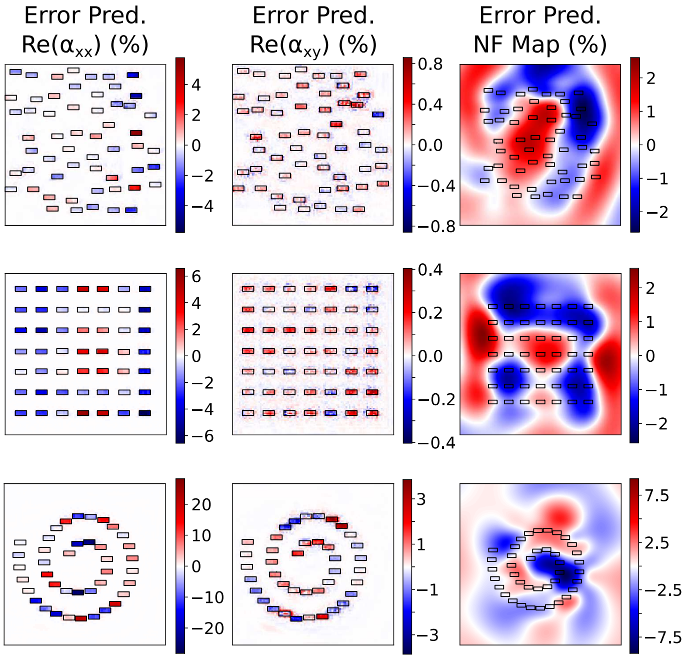


Figure S5. Error maps of the examples shown in main text figure 4.

We show in figure S5 colormaps of the prediction errors for the examples shown in the main text Figure 4.

### E. Local approximation: Impact of window size

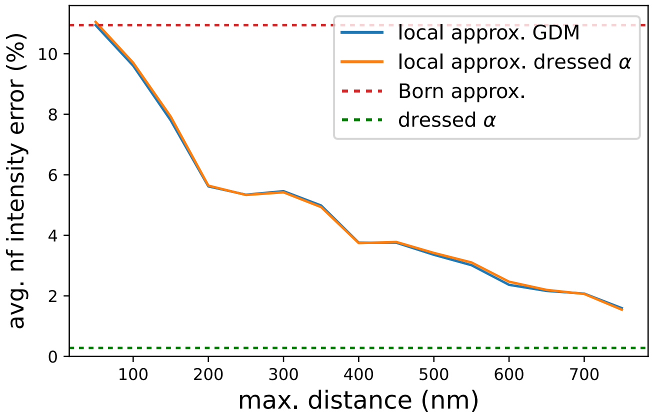


Figure S6. Error of the local neighborhood approximation on the near-field calculation as function of the window size in which optical interactions are taken into account.

Figure S6 shows the approximation error if optical interactions for gold rods at larger distances are neglected. The shown results are all based on numerical calculations, no neural network prediction is shown here. The Born approximation (red dashed line) corresponds to the case of no optical interactions, the curve labeled "dressed $\alpha$" (green dashed line) corresponds to an unlimited interaction radius. The error is relative to the full field simulation with all interactions included. We also compare the local approximation dressed polarizabilities (orange solid line) to the local approximation with full field simulations (blue solid line), which again shows an excellent agreement between the methods.

### F. Qualitative benchmark of spectral predictions

For a direct comparison with sections II-IV of the main paper, we also trained a spectral network on the $70 \times 30 \times 30\,\mathrm{nm}^3$ gold nano-rod geometry.

In figure S7 we show examples of spectral predictions for different arrangements of five identical elongated gold nano-rods. The left column displays the geometric arrangement in the $XY$ plane. The second and third columns show respectively the real and imaginary part of $\alpha_{xx}$. The fourth column shows the far-field scattering cross section obtained via re-propagation of the electric dipole moments of the five scatterers after illumination with an $X$-polarized, normally incident plane wave. At the very right, the effective dipole moments of the rods under the $X$-polarized illumination are indicated by small arrows for selected wavelengths. The colors of the lines and of the arrows correspond to the color-code defined in the geometry panel in the left column. Solid lines indicate the network's prediction, dashed lines show the simulated results. For comparison, the response of an isolated gold-rod is indicated by black dotted lines in all figures. From a first observation of the predicted spectra we find an excellent agreement of the simulated and neural network predicted polarizabilities over the entire wavelength range. Also the derived far-field scattering is in an excellent agreement with the GDM simulations.

Figure S7a shows a random distribution of the five rods, similar to the structures in the training data. The random distribution results in a relatively weak modification of the individual dressed polarizabilities. The main observation is a broadening and slight red-shift of the localized plasmon resonance, which is apparent in particular in the far-field scattering spectrum (see panel on the very right). The red-shift can be explained in a qualitative picture by the presence of the neighbor nano-rods which increase the local effective index. The disordered arrangement inhibits efficient optical coupling of rods. Fig. S7b shows an entirely different configuration: The five rods are aligned as a chain, with equidistant gaps of 20 nm. In this case, the dressed polarizabilities have a significantly different spectral shape. At the resonance wavelength of the isolated nano-rod, the phase of the dipole moment has flipped its sign (c.f. $\mathrm{Re}(\alpha_{xx})$) and the peak of the resonance has shifted quite drastically to a wavelength around $\lambda = 690\,\mathrm{nm}$ (c.f. $\mathrm{Im}(\alpha_{xx})$). We furthermore observe a significant increase in the scattering efficiency at that wavelength, being around twice as high (per nano-rod), compared to the single scatter. This is a result of the collective, resonant excitation of all five rods, as can be seen in the sketch on the right. Additionally we observe a second small peak in the far-field

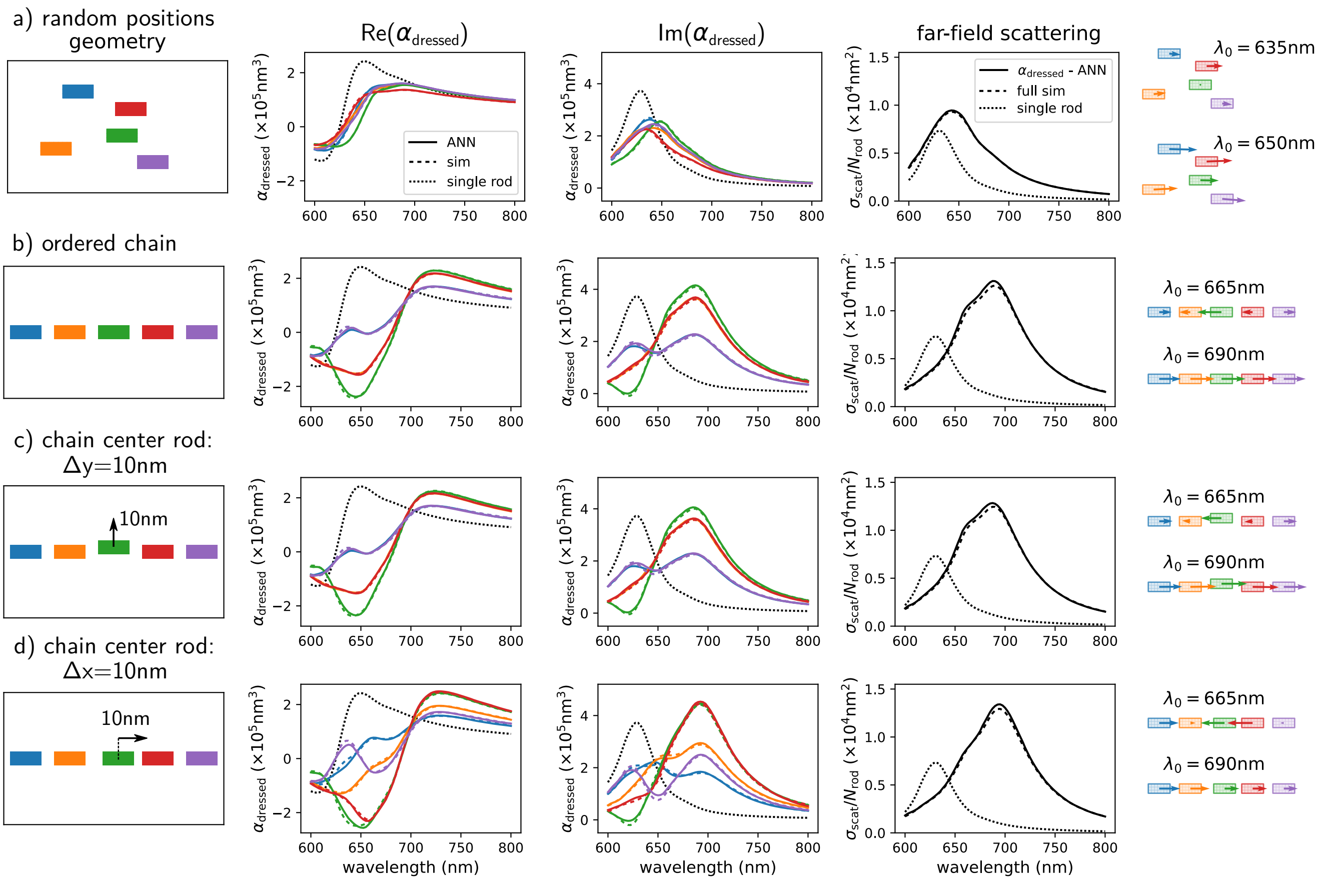


Figure S7. Spectral dressed polarizability predictions compared to simulations. a) Random distribution of 5 gold rods. b) Ordered chain of 5 gold nano-rods with an equal spacing of 20 nm to one another. c) same chain as in (b) but with the center rod being displaced by 10 nm towards out of the chain. d) same chain as in (b) but with the center rod being displaced by 10 nm along the chain's axis towards the right neighbor. The areas in the left panels are $500 \times 300\,\mathrm{nm}^2$ in size. The second-left column shows the real part of the $\alpha_{xx}$ component, the second-right column the respective imaginary part. The color codes in those panels assign the polarizability curves to the according rods of same color in the geometry views on the very left. Solid lines correspond to the network predictions, and dashed lines indicate the simulations. In the second right column we show spectra of the scattering cross-section divided by the number of rods, calculated with normally incident plane waves of linear polarization along $X$, either with the predicted dressed polarizabilities (solid lines) or via full simulations (dashed lines). For comparison, the results for an isolated nano-rod are shown in all plots as black dotted line. On the very right, the real parts of the effective electric dipole moments are shown at selected wavelengths, as indicated by the respective labels.

scattering at around $\lambda_0 = 665\,\mathrm{nm}$. A closer inspection of the distribution of effective dipole moments reveals that this second resonance corresponds to a kind of anti-bonding mode, where the outer gold-rods oscillate with an opposite phase compared to the center rods, as can be seen in the according sketch on the very right of Fig. S7b.

In the figures S7c-d we study the impact of a small distortion in the chain of plasmonic nano-rods. Figure S7c shows the polarizabilities and far-field scattering for the same chain as in Fig. S7b, with the only difference that the center gold rod was moved by 10 nm towards $Y$, perpendicular to the chain's long axis. We find in the analysis of the dressed polarizabilities as well as in the far-field spectrum, that this distortion has no significant effect on the optical response. On the other hand, if we move the same nano-rod by 10 nm *along* the chain's axis (towards positive $X$, shown in Fig. S7d), the effect is surprisingly more dramatic. This small change in the geometry strongly modifies the dressed polarizabilities of the rods. It breaks the symmetry of the formerly identical rod pairs on the left and right of the chain, and in the far-field the red-shift of the resonance is further increased while the double-peak, which was present in the full-chain is suppressed. An analysis of the effective dipole moments at the wavelength of the former anti-bonding mode reveals that the asymmetric excitation leads to an exaltation of the shifted nano-rod's dipole moment (green) as well as of it's closest neighbor (red), which is breaking the anti-bonding mode's symmetry. At the peak resonance around $\lambda_0 = 690\,\mathrm{nm}$ however, the rods in the chain are still fully oscillating in phase, resulting in efficient far-field scattering.

## G. Statistics of spectrally resolved predictions

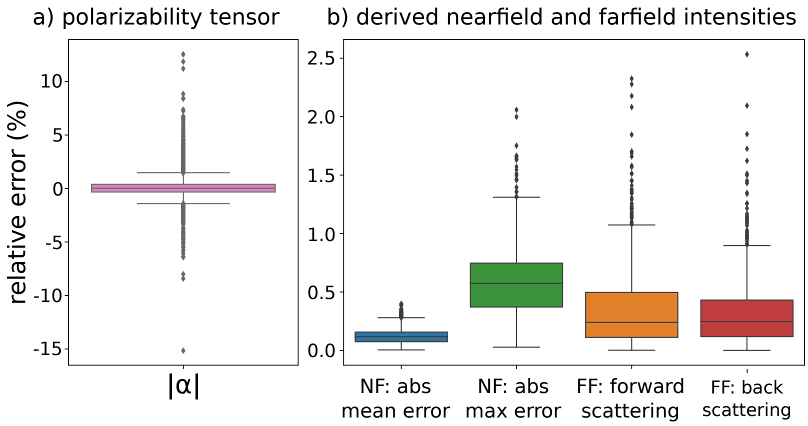


Figure S8. Statistics of the spectral predictor on 1000 random arrangements of gold rods. a) accuracy of the polarizabilitiy tensor norm for all individual gold rods. b) accuracy of derived near- and far-field intensity.

Figure S8 shows the statistics of the network trained on the spectrally resolved dataset with the $70 \times 30 \times 30\,\mathrm{nm}^3$ gold nano-rods. In comparison to the fixed-wavelength network we find similar trends for the errors of the different quantities, and even overall slightly better accuracy in the spectral case which we attribute to the significantly larger size of the training dataset (150000 samples in the spectral case vs 60000 for the single-wavelength network).

In order to corroborate why the spectral network performs better than the single-wavelength predictor, we trained a further network on a data-set of 60000 samples using the same area as used for the spectral training ($600 \times 600\,\mathrm{nm}^2$), but restricted to the resonance wavelength $\lambda_0 = 635\,\mathrm{nm}$ of a single nano-rod (on glass substrate). After training on this data, we obtain a predictor accuracy in the same order as for the spectral dataset. We conclude that the size of the input area has a stronger impact on the prediction fidelity than the addition of the wavelength as additional degree of freedom.

[S1] S. Ioffe and C. Szegedy, arXiv:1502.03167 [cs] (2015), arXiv:1502.03167 [cs].
[S2] A. L. Maas, A. Y. Hannun, and A. Y. Ng, in *Proceedings of the 30th International Conference on Machine Learning* (Citeseer, Atlanta, USA, 2013).
[S3] D. P. Kingma and J. Ba, arXiv:1412.6980 [cs] (2014), arXiv:1412.6980 [cs].
[S4] S. L. Smith, P.-J. Kindermans, C. Ying, and Q. V. Le, arXiv:1711.00489 [cs, stat] (2018), arXiv:1711.00489 [cs, stat].
[S5] F. Chollet, *Deep Learning with Python* (Manning Publications Company, 2017).
